# Supplementary material for: Twelve Scientific Challenges for 6G: Rethinking the Foundations of Communications Theory
Source: arXiv:2207.01843 source file (2023-02-08)
Supplement: Supplementary file 1 [file appendixA.tex]

\appendix

\subsection{Appendix A}\label{sec:AppA}
